# Supplementary material for: Autonomous Electron Tomography Reconstruction with Machine Learning
Source: arXiv:2308.00099 source file (2023-09-08)
Supplement: Supplementary file 1 [file 20230720_supplemental_materials_Autonomous_electron_tomography_reconstruction_with_machine_learning.pdf]

Supplemental Materials:

Autonomous Electron Tomography Reconstruction with Machine Learning

William Millsaps, Jonathan Schwartz, Zichao Wendy Di, Yi Jiang, Robert Hovden

This document outlines the Python code to run Bayesian Optimization for hyperparameter selection compressed sensing tomography. There are two files, bayesian_tomography.py and simulation_utils.py, which contain the essential components. bayesian_tomography.py runs Bayesian Optimization and can be customized, and simulation_utils.py provides initialization and the FISTA reconstruction algorithm. However, to run our tomography reconstruction code (astra_ctvlib), the github repository must also be cloned and compiled or additional reconstruction codes should be imported from elsewhere (e.g. tomopy or PyHST2). To port additional reconstruction algorithms or functions of interest, ignore pages 1-4 and edit line 27 on page 5 (where the reconstruction_object is created) to implement BO for additional applications.

```
##### Clone https://github.com/hovdenlab/Autonomous_Tomography_BO for astra_ctvlib and pytvlib #####

##### simulation_utils_FISTA.py #####
    #Originally Written for Python version: 3.8.10

##### Import Modules #####
import gpu_3D.Utils.astra_ctvlib as astra_ctvlib
import gpu_3D.Utils.pytvlib as pytvlib
from tqdm import tqdm
import numpy as np
import h5py

class FISTA_simulation:

    def __init__(self, fname,tiltAngles, SNR=5):

        # Load the Original Volume (customize this per input file type)
        file = h5py.File(fname,'r')
        self.original_volume = file['recon'][:]
        file.close()

        # Read Dimensions of Test Object
        (self.Nx, self.Ny, self.Nz) = self.original_volume.shape
```

```
# Initialize the C++ Object
self.tomography_object = astra_ctvlib.astra_ctvlib(self.Nx, self.Ny,
np.deg2rad(tiltAngles))

## astra_ctvlib by default creates one 3D volume for the reconstruction, any additional
volumes needs to be externally intialized (this is to save memory consumption) ##
self.tomography_object.initialize_initial_volume()

# Optional: Apply Poisson Noise to Background Volume
self.original_volume[self.original_volume == 0] = 1

# Let's pass the volume from python to C++
for s in range(self.Nx):
    self.tomography_object.set_original_volume(self.original_volume[s,:,:],s)

# Now Let's Create the Projection Images
self.tomography_object.create_projections()

# Optional: Apply poisson noise to volume
if SNR != 0: self.tomography_object.poisson_noise(SNR)


        ### Perform FISTA reconstruction ###

def FISTA_recon(self, params):

    # Initialize Reconstruction
    self.tomography_object.restart_recon()
    self.rmse_vec, self.dd_vec, self.tv_vec = np.zeros(params['Niter']),
    np.zeros(params['Niter']), np.zeros(params['Niter'])

    # Inialize the Reconstruction Algorithm
    alg = params['alg']
    pytvlib.initialize_algorithm(self.tomography_object,alg)

    # Reconstruction Parameters
    self.params = params
    lambdaParam = params['lambdaParam']; Niter = params['Niter']; nTViter =
    params['nTViter']

    # Momentum and Objective Function
    self.fista_cost = np.zeros(Niter); t0 = 1
```

```
        ### Main Loop ###
        for k in tqdm(range(Niter)):

            # Gradient Step
            pytvlib.run(self.tomography_object,alg)

            # Threshold Step
            self.tomography_object.tv_fgp(nTViter,lambdaParam)

            # Momentum Step
            tk = 0.5 * (1 + np.sqrt(1 + 4 * t0**2))
            self.tomography_object.fista_momentum((t0-1)/tk)
            t0 = tk

            # Measure Objective
            self.fista_cost[k] = 0.5 * self.tomography_object.data_distance()**2 + lambdaParam *
            self.tomography_object.tv()

            # Measure other performance metrics

            self.dd_vec[k] = self.tomography_object.data_distance()
            self.tv_vec[k] = self.tomography_object.tv()
            self.rmse_vec[k] = self.tomography_object.rmse()

        # Return the Reconstruction to Python
        self.recon = np.zeros([self.Nx, self.Ny, self.Nz],dtype=np.float32)
        for s in range(self.Nx):
            self.recon[s,] = self.tomography_object.get_recon(s)

        return [self.tomography_object.rmse()]

    def save_results(self,fname, groupName, i):
        h5File = h5py.File(fname,'a')
        group = h5File.create_group(groupName+'/'+str(i))
        group.create_dataset('LambdaParam', data=self.params['lambdaParam'])
        group.create_dataset('RMSE', data= self.rmse_vec)
        group.create_dataset('Reconstruction', data=self.recon[140,:,:])
        group.create_dataset('DD',data=self.dd_vec)
        group.create_dataset('TV',data=self.tv_vec)
        group.create_dataset('FISTA_cost',data=self.fista_cost)
        h5File.close()
```

```
##### Bayesian Optimization #####

##### bayesian_tomography.py #####
        #Originally Written for Python version: 3.8.10

##### Import Modules #####

from skopt import Optimizer
from skopt.space.space import Real
from skopt.plots import plot_gaussian_process
from sklearn.gaussian_process.kernels import Matern
from skopt.learning import GaussianProcessRegressor as GPR
import simulation_utils_FISTA
import random
import numpy as np
from datetime import datetime
import matplotlib.pyplot as plt
import os

##### Prepare reconstruction script #####

# Test Phantom Object
filename = 'your_file'

# Tilt Series for Experiment / Simulation
tiltAngles = np.arange(-70,70,2)
recon_parameters = {'lambdaParam':0, 'Niter': 100, 'nTViter':15, 'alg':'fista'}

# Class for Performing Reconstructions
reconstructor_object = simulation_utils_FISTA.FISTA_simulation(filename,tiltAngles)

# BO Parameters
nBOiter = 20      # Total iterations (including initial pts)
lower_bound = 1
upper_bound = 5000
n_init_pts = 5
nu = 2.5      # nu controls the smoothness of the matern kernel fitting for GP (e.g. nu = 1.5
corresponds to once differentiable functions, and nu = 2.5 to twice differentiable functions).

##### Prepare optimizer #####
```

```
# Define the Kernel
mat_kern = Matern(length_scale = 1, length_scale_bounds = (1, 10), nu = nu)
gpr = GPR(kernel = mat_kern, n_restarts_optimizer = 10)

# Define bounds for fit parameter
bounds = [Real(lower_bound, upper_bound, name = 'lambda')]
initial_sampling = np.linspace(lower_bound,  upper_bound, n_init_pts)
init_pts_generator = 'grid'

# Optimizer for BO
rng_seed = int(datetime.now().strftime('%f'))
random.seed(rng_seed)
opt = Optimizer(bounds, base_estimator = gpr, acq_func = 'gp_hedge',n_initial_points = n_init_pts,
initial_point_generator=init_pts_generator, acq_optimizer='sampling',random_state=rng_seed)

# Parameters for plotting and saving Bayesian predictions
save_directory = 'Bayesian_Optimization_tomography/' # Your results folder
fname = 'lambdaParam_tuning.h5' # File with results
output_name = 'lambdaParam_explore' # h5 group name
if not os.path.exists(save_directory): os.makedirs(save_directory) # Make directory
kwargs = {'show_acq_func' :False, 'show_mu' :True, 'show_legend': False} # Optional arguments for
plotting

# Main Loop
for i in range(nBOiter):

    # Ask optimizer for next parameter to evaluate
    next_lambda = opt.ask()[0]
    recon_parameters['lambdaParam'] = next_lambda

    # Perform reconstruction, evaluate the performance (this function call can be replaced for any
general black box function of interest)
   data_error = reconstructor_object.FISTA_recon(recon_parameters)

    # Tell the optimizer the result of the reconstruction
    res = opt.tell([next_lambda], data_error)

    # Save data of interest:
    reconstructor_object.save_results(save_directory+fname, output_name, i+1)         # Save 2D
slices from the reconstruction
```

```
# Save plot of Bayesian Optimization
if i >= n_init_pts:
    plt.figure()
    plot_gaussian_process(res,**kwargs)     # Recreate Parameter Estimate Plots from Fig. 3a
    plt.savefig(f'{save_directory}bo_gp{i+1}.png', transparent = False, bbox_inches = 'tight')
```
